# Supplementary material for: Grammar-Constrained Decoding for Structured NLP Tasks without Finetuning
Source: arXiv:2305.13971 source file (2024-01-18)
Supplement: Supplementary file 1 [file 06_experiment_settings_CP.tex]

\section{CP Task Settings}\label{app_sec:constituency_parsing}

\subsection{Dataset Preprocessing}\label{appendix:dataset-preprocessing}

\subsection{Out of Knowledge Base Mention}\label{appendix:out-of-kb-mention}
%It's important to note that some of these datasets contain mentions that are not present in the knowledge base (YAGO\_KB)
%To ensure consistency and accuracy, we filter out these mentions, exclusively utilizing the ones that are available.
%
%We report the number of data points whose target entity is not in the knowledge base. The number of data points is reported for each dataset.
%
%\begin{itemize}
%    \item AIDA-CoNLL: 0 out of 4485
%    \item ACE2004: 0 out of 257
%    \item AQUAINT: 4 out of 727
%    \item ClueWeb: 12 out of 11154
%    \item MSNBC: 0 out of 656
%    \item Wikipedia: 23 out of 6821
%%    \item UnseenMention(wikilinksNED): 2616 out of 10000
%\end{itemize}
%
%These data points are filtered out in the experiments with input-independent grammar.
%
%In the experiments with input-dependent grammar, we filter out the data points whose candidate set is empty.
%\begin{itemize}
%    \item AIDA-CoNLL: 0 out of 4485
%    \item ACE2004: 17 out of 257
%    \item AQUAINT: 24 out of 727
%    \item ClueWeb: 44 out of 11154
%    \item MSNBC: 5 out of 656
%    \item Wikipedia: 7 out of 6821
%    \item UnseenMention(wikilinksNED): 114 out of 10000
%\end{itemize}

\subsection{Metrics}
%
%Many previous works~\cite{decao2021autoregressive, ganea2017deep, ayoola-etal-2022-refined} report the micro-averaged F1 score from Gerbil evaluation tool.
%In our approach, we always take the top-1 prediction as the final prediction.
%Since each mention is only associated with one target entity, the micro-averaged F1 score is equivalent to the accuracy in this case (accuracy = precision = recall = F1)
%We report the accuracy as the evaluation metric for the ED task and didn't use Gerbil evaluation tool.
