# Supplementary material for: Grammar-Constrained Decoding for Structured NLP Tasks without Finetuning
Source: arXiv:2305.13971 source file (2024-01-18)
Supplement: Supplementary file 2 [file cp_main_results_more.tex]

\begin{table}[h]
\centering
\resizebox{0.48\textwidth}{!}{
\setlength{\tabcolsep}{5pt}
\begin{tabular}{@{}lccccc@{}}
\toprule
\hspace{4mm} Method & Precision & Recall & Tag Accuracy & F1 & Validity \\
\midrule
\emph{\textbf{Unconstrained}}\\
\hspace{4mm} LLaMA-7B      &    30.2     &    26.3     &    30.3  & 28.1 &    54.3 \\
\hspace{4mm} LLaMA-13B     &    45.9     &    40.1     &    37.1  & 42.8 &    69.4 \\
\hspace{4mm} LLaMA-33B     &    46.1     &    40.1     &    42.3  & 42.9 &    64.2 \\
\midrule
\emph{\textbf{Constrained IIG}}\\
\hspace{4mm} LLaMA-7B      &    37.4     &    32.3     &    35.2  & 34.7 &    65.9 \\
\hspace{4mm} LLaMA-13B     &    48.6     &    42.6     &    39.9  & 45.4 &    80.3 \\
\hspace{4mm} LLaMA-33B     &    48.6     &    45.6     &    44.5  & 47.1 &    72.3 \\
\midrule
\emph{\textbf{Constrained IDG}}\\
\hspace{4mm} LLaMA-7B      &    51.0     &    41.6     &    45.0  & 45.8 &    100.0 \\
\hspace{4mm} LLaMA-13B     &    56.8     &    50.3     &    44.2  & 53.4 &    100.0 \\
\hspace{4mm} LLaMA-33B     &    \textbf{57.5}     &    \textbf{51.9}     &    \textbf{51.0}  & 54.6 &    \textbf{100.0} \\
\bottomrule
\end{tabular}
}
\caption{\textbf{Main results for constituency parsing (8 shots)} We report the precision, recall and validity of the parse trees on the SynthIE-text test subset (only gold parse trees shorter than 64 tokens are used).
The width of the \textbf{confidence intervals (90\%)} are between 4.0 and 6.0 for all results except the validity of the constrained models, which is constant. The best results are in bold.}
\label{tab:ConstituencyParsingResultsMore}
\end{table}
